# Supplementary material for: Who is a Better Talker: Subjective and Objective Quality Assessment for AI-Generated Talking Heads
Source: arXiv:2507.23343 source file (2025-07-31)
Supplement: Supplementary file 1 [file X_suppl.tex]

\clearpage
\setcounter{page}{1}
\maketitlesupplementary

\section{Subjective Assessment Interface \& Details}
In order to facilitate subjects' subjective assessment of AGTHs in THQA-10K and subsequent data submission and collection, we design a subjective scoring interface for this subjective experiment by combining \textit{Python} and \textit{Gradio}, as shown in Fig.~\ref{fig:gui}. The left side of Fig.~\ref{fig:gui} shows the ``Video" area, which is used to present the AGTHs, while the right side is the subjective scoring area, which includes two dimensions, namely, distortion type and overall quality score. In particular, the distortion type is set as a multiple choice box to more comprehensively label the distortions occurring in the AGTHs. On the first day of subjective experiment, all participants participated in a training session lasting approximately 30 minutes. During this session, they were told to assess the quality of each AGTH using the Absolute Category Rating (ACR) method and instructed on how to recognize the type of distortion present in each AGTH. Subsequently, participants were shown the assessment interface and were given sufficient time to familiarize themselves with the scoring procedures.

\begin{figure}[!h]
    
    \centering
    \includegraphics[width =0.95\linewidth]{pic/gui.png}
    \vspace{-0.2cm}
    \caption{The Gradio-based quality assessment website, designed for multi-distortion categorization and quality rating.}
    \label{fig:gui}
    \vspace{-0.6cm}
\end{figure}
\section{Limitation \& Solution}
Although the proposed FSCD method achieves state-of-the-art performance on THQA-10K, THQA and THQA-3D datasets, it has some limitations: L1) FSCD relies on the generated image frames for the detection of the centre point of the face's mouth, which puts certain requirements on both the generated portrait image and the face keypoint detection algorithm. requirements. In extreme cases, such as when the image quality of the AGPI is too low to detect a face, FSCD cannot be used directly.L2) Although slicing the mouth centroids against the AGTHs is a simple implementation, it may not be optimal. To cope with these two limitations, we optimise and outlook the FSCD method: S1) For the special case of AGPIs where face detection fails, we fix the x-coordinate of the mouth centroid directly at 1/2 width of the AGPIs image. In order to verify the reasonableness of this method, we perform statistical analysis for the mouth centroids of all AGPIs that successfully detected faces, and the results are shown in Fig.~\ref{fig:pos}. Fig.~\ref{fig:pos} clearly shows that the vast majority of AGPIs in the two generative speaker head quality assessment datasets THQA-10K and THQA have the face in the middle of the frame, and even more so, the authors of THQA-3D aimed the viewpoint at the centre of the head model when rendering the 3D speaker head model as a video. Therefore, it is statistically significant that the position of the centre of the mouth is of maximum likelihood probability when it is at 1/2 image width in the case of a failed face detection. S2) The choice of tangent location and form is an issue worth exploring. In addition to slicing AGTHs through the mouth centroid in the form of a Y-T slice, more adaptive methods may provide richer quality features.

\begin{figure}[!h]
    \centering
    
    \subfloat[THQA-10K dataset]{\includegraphics[width=\linewidth]{supppic/thqa10kpos.pdf}}

    \subfloat[THQA dataset]{\includegraphics[width=\linewidth]{supppic/thqa800pos.pdf}}
    
    \vspace{-0.3cm}
    \caption{The x-axis position of the centre point of the faces of the different AGPIs as they appear, with brighter locations indicating a higher number of occurrences. All AGPIs are scaled isometrically to 1,024 × 1,024 resolution.}
    \label{fig:pos}
    \vspace{-0.6cm}
\end{figure}

\section{Reference}
